# Supplementary material for: Digital Twin Buildings: 3D Modeling, GIS Integration, and Visual Descriptions Using Gaussian Splatting, ChatGPT/Deepseek, and Google Maps Platform
Source: arXiv:2502.05769 source file (2025-04-20)
Supplement: Supplementary file 1 [file 7appendix.tex]

\newpage
\appendix % Start Appendix

 % Figure numbering as A1, A2, etc.
   % Table numbering as A1, A2, etc.
\setcounter{figure}{0}  % Reset figure counter
\setcounter{table}{0}   % Reset table counter

\section*{Additional Results}
The per-scene-per-model average CLIP scores are shown in Fig. \ref{fig:4ModelsCaptionCLIp_perbuilding}. Deepseek-V3 achieves higher caption CLIP scores than other LLMs, except in two cases. The first is the ICON scene, which features twin high-rise buildings with retail spaces at the ground level. The second is the Parliament Hill of Canada scene overlooking the Ottawa River, characterized by its gothic-style architecture. Notably, the Parliament Hill scene also received the lowest overall CLIP scores.

\begin{figure*}[htpb]
\centering
\includegraphics[width = 0.9\textwidth]{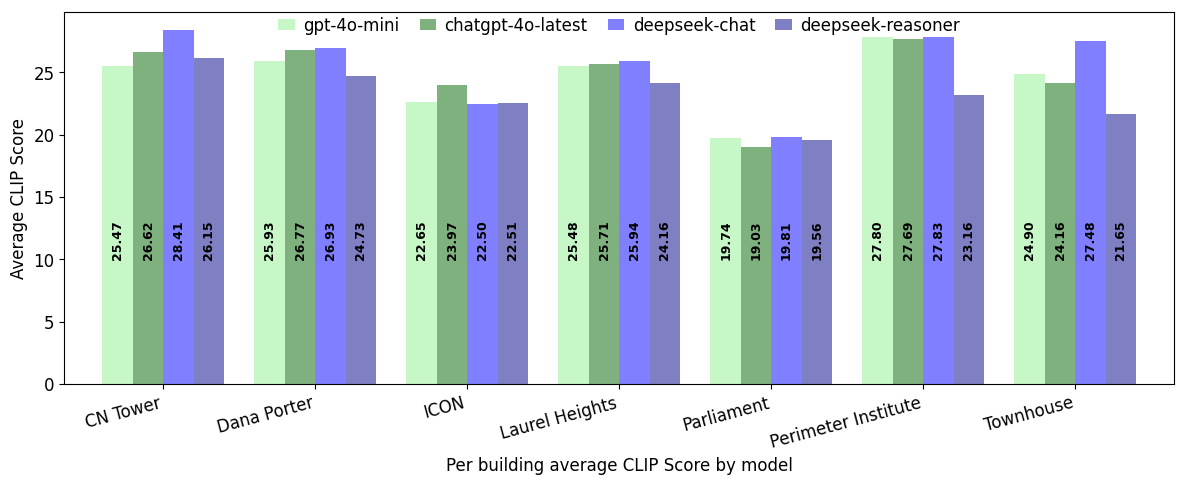}
\caption{Average CLIP score of each building image captioning model for each different scene.}\label{fig:4ModelsCaptionCLIp_perbuilding}
\end{figure*}

\section*{Input images}
Input images for the Parliament Hill scene (Fig. \ref{fig:parliament_hill}) and the ICON scene (Fig. \ref{fig:icon}) are provided. These are the two scenes with the lowest multi-agent captioning CLIP scores. 
\begin{figure}[h]
    \centering
    \begin{subfigure}{0.15\textwidth}
        \includegraphics[width=\linewidth]{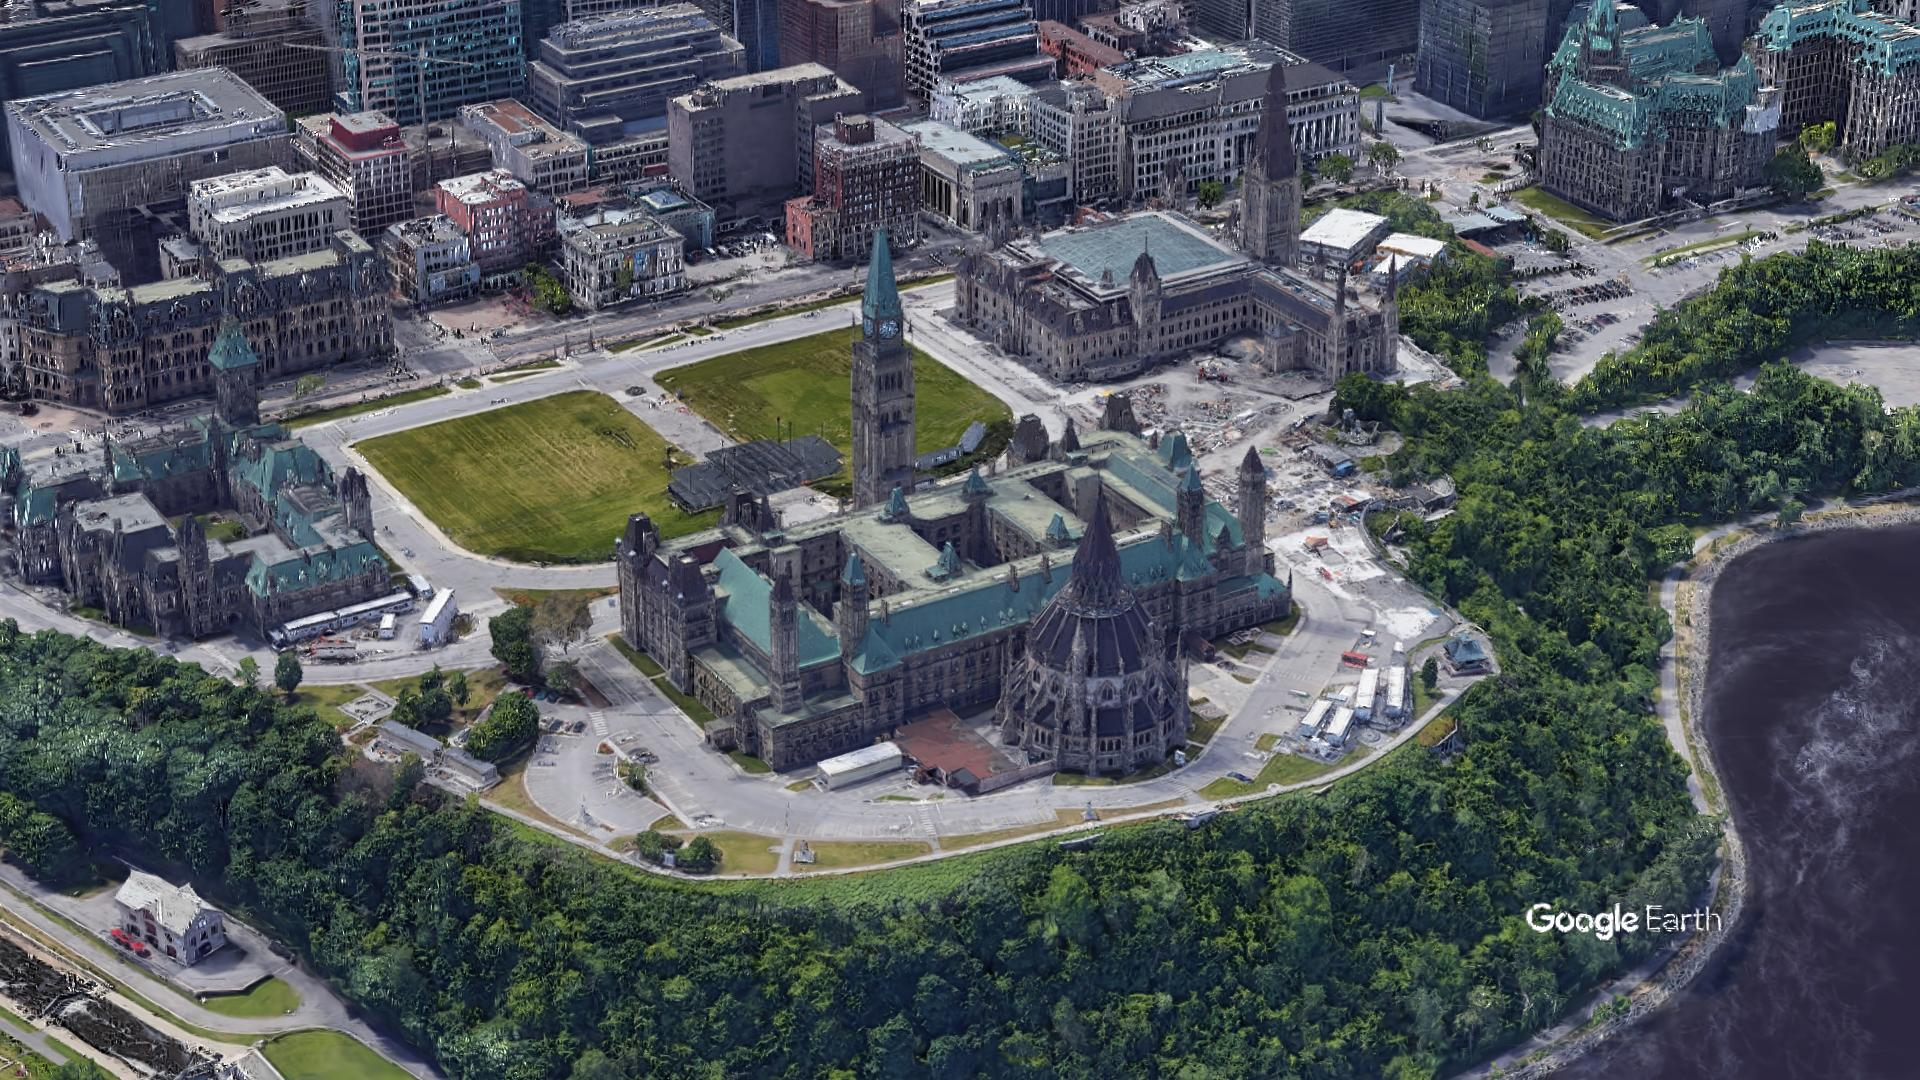} 
    \end{subfigure}
    \begin{subfigure}{0.15\textwidth}
        \includegraphics[width=\linewidth]{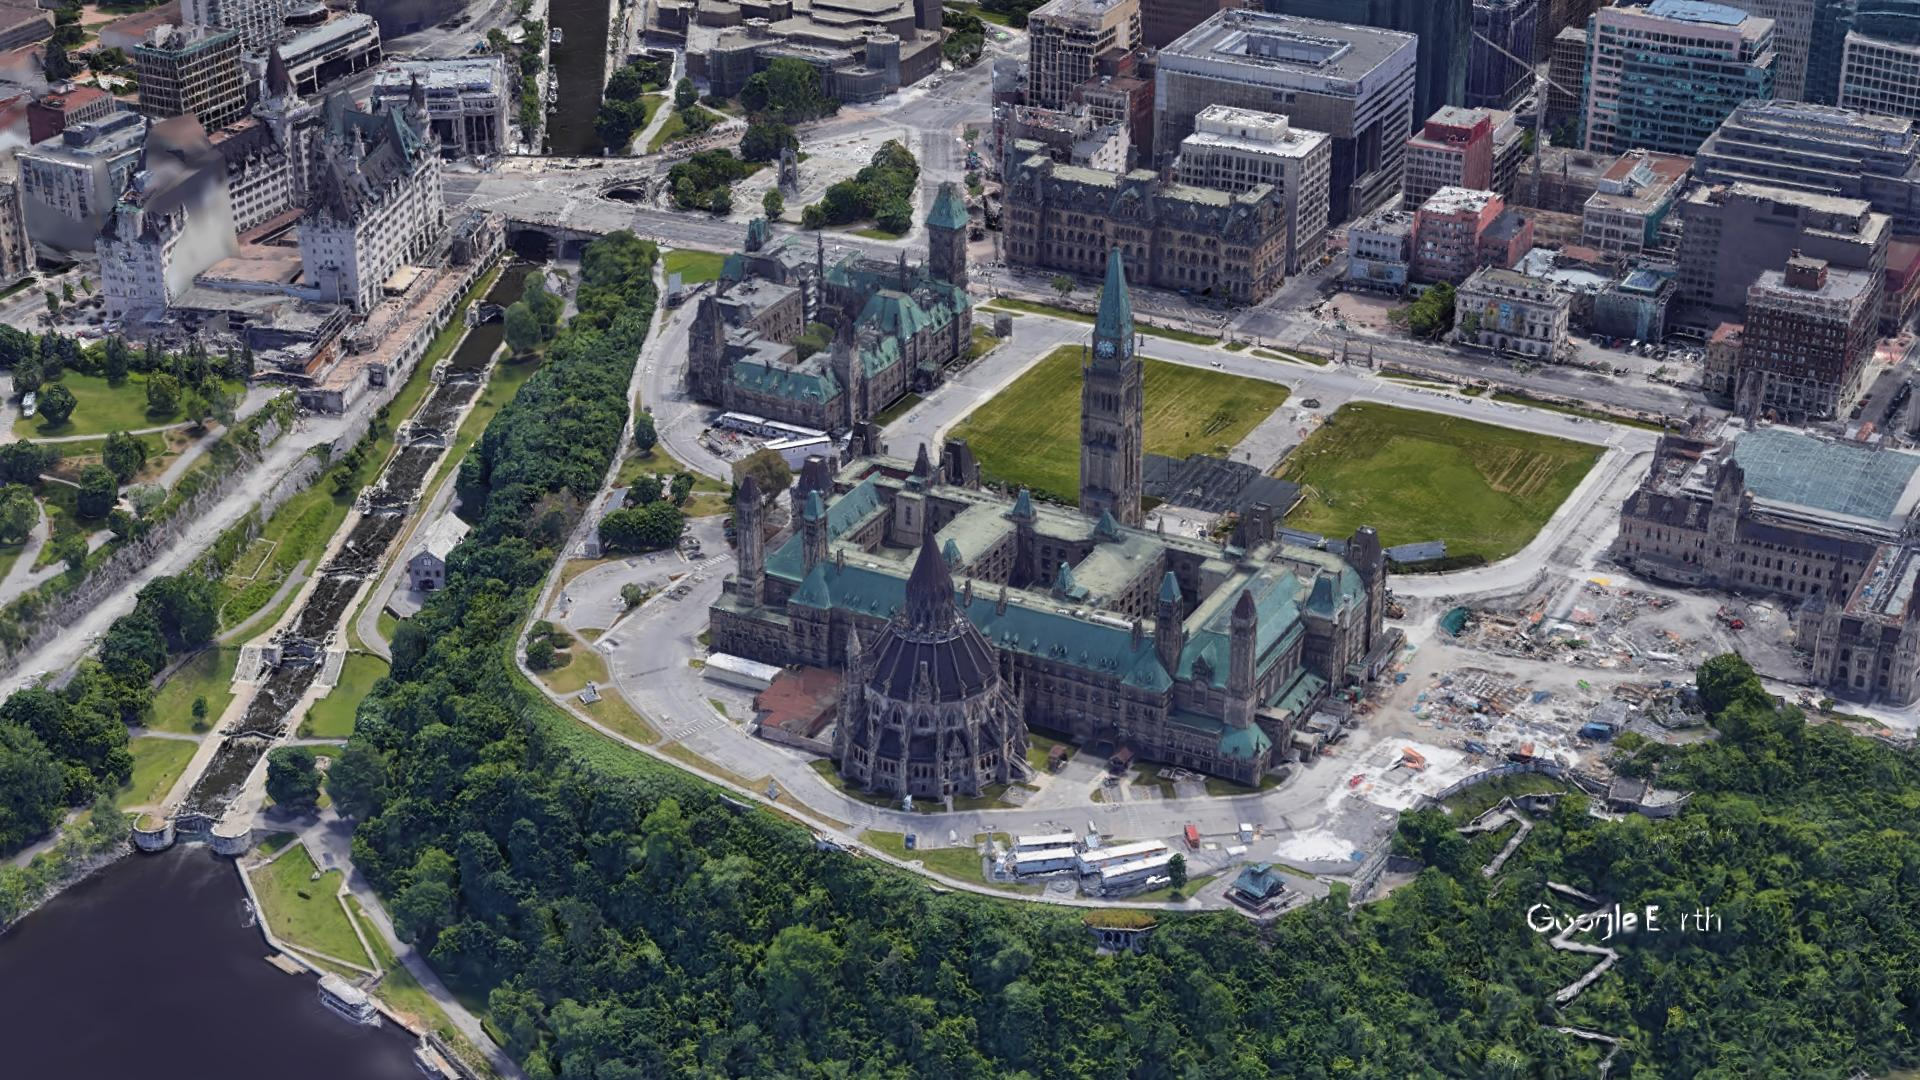}
    \end{subfigure}
    \begin{subfigure}{0.15\textwidth}
        \includegraphics[width=\linewidth]{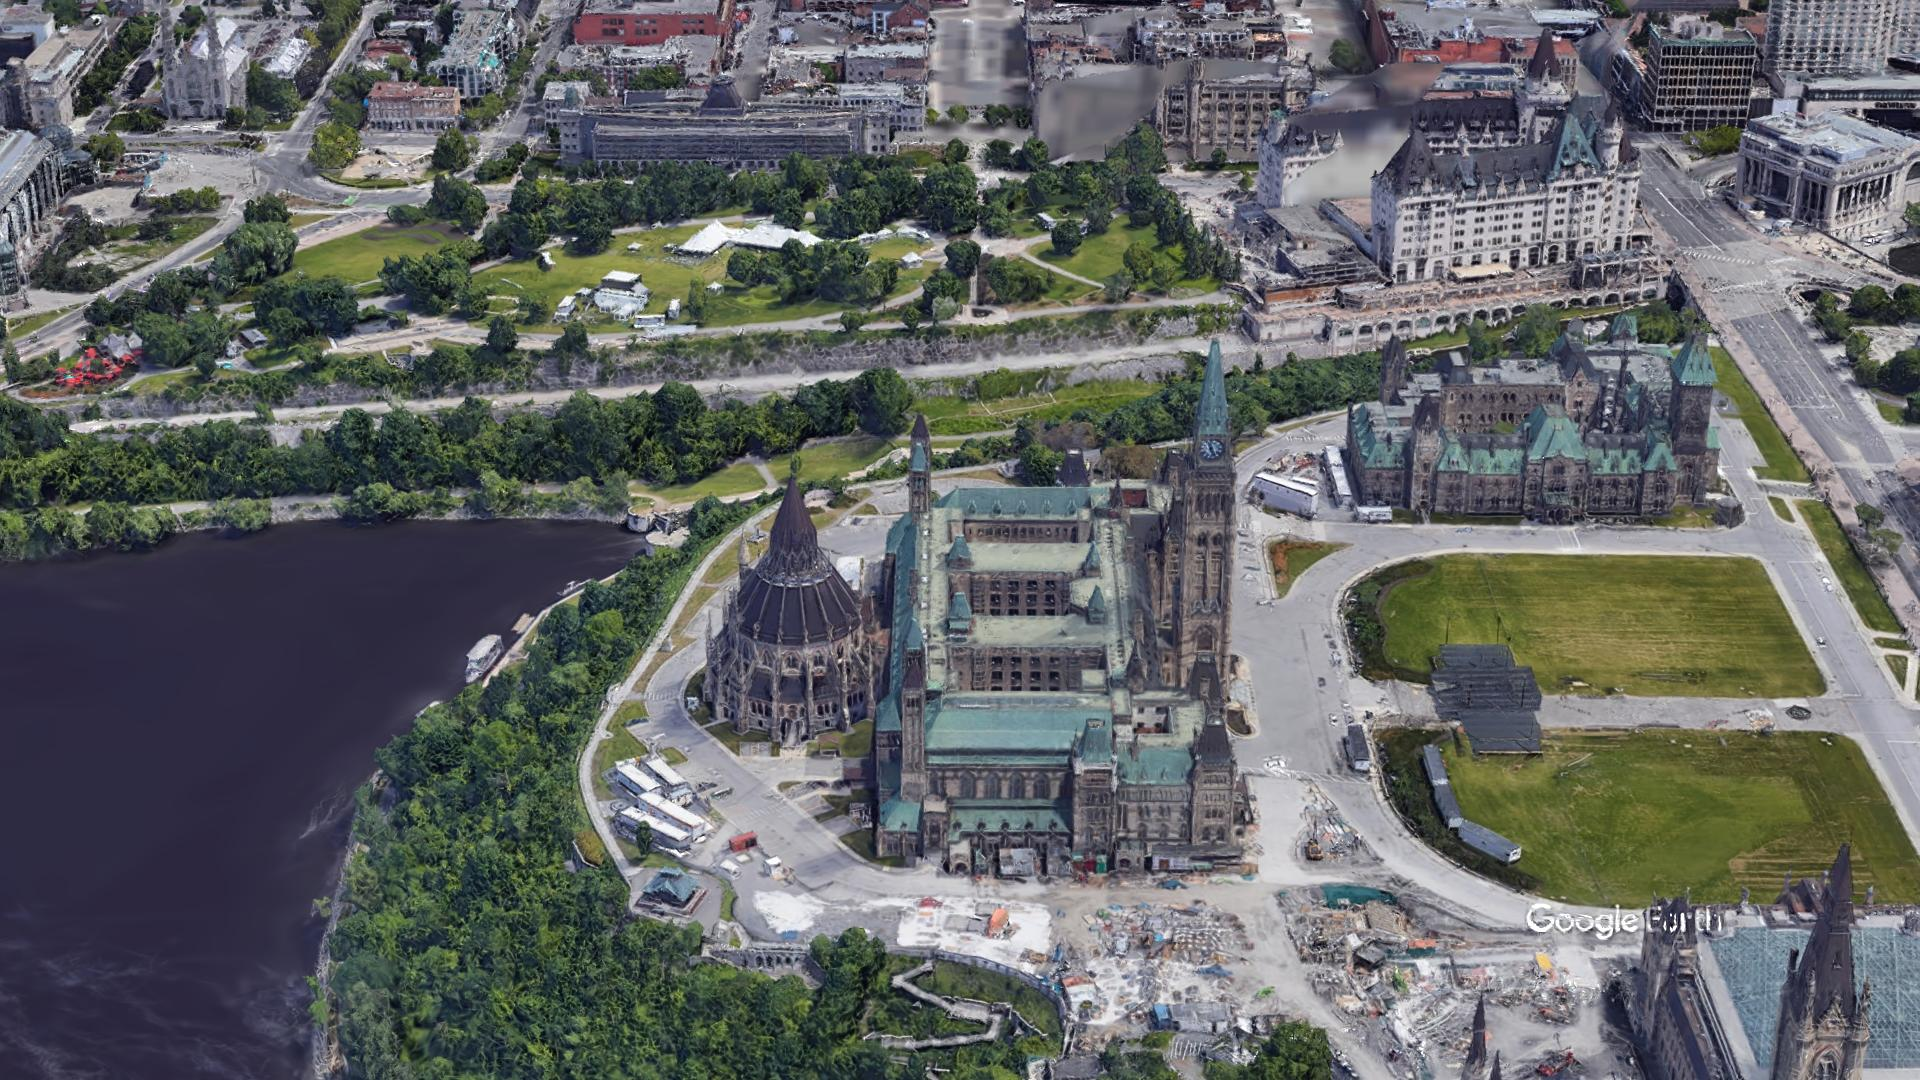}
    \end{subfigure}
    \\
    \begin{subfigure}{0.15\textwidth}
        \includegraphics[width=\linewidth]{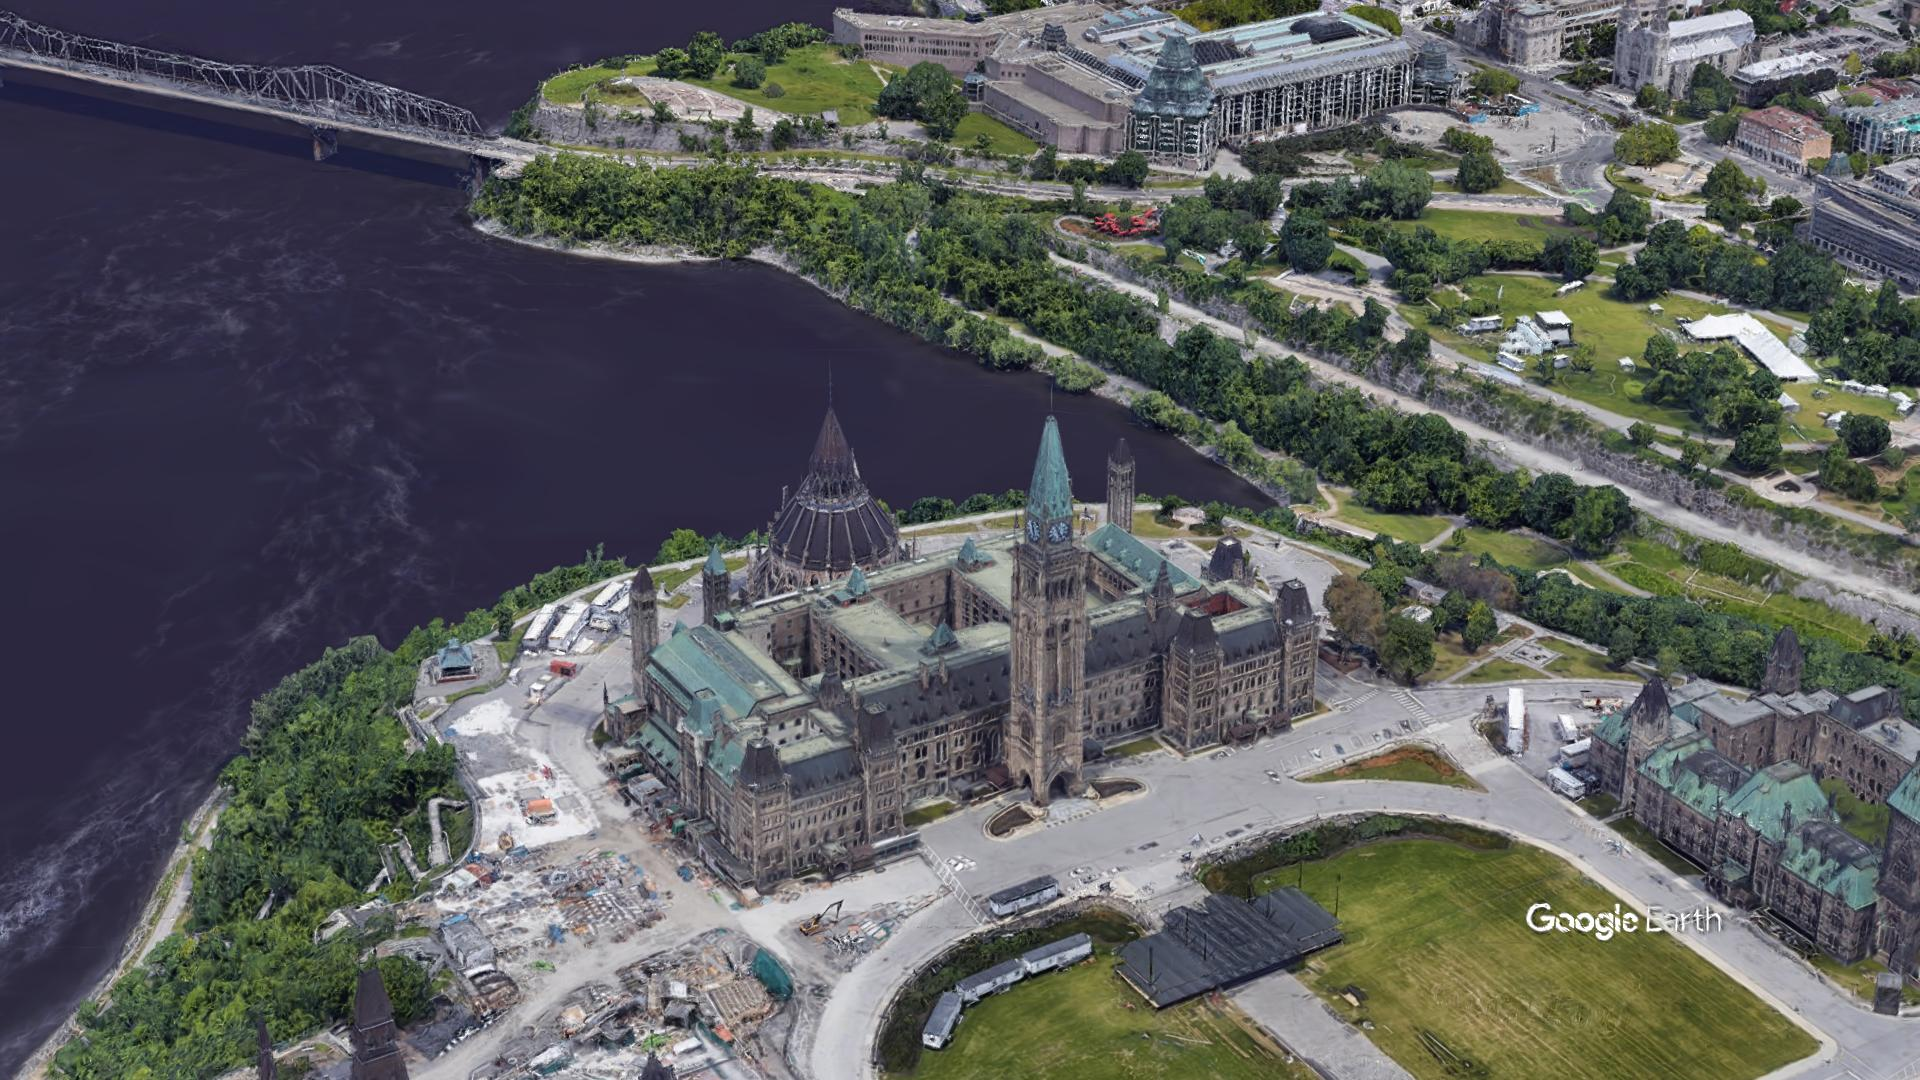}
    \end{subfigure}
    \begin{subfigure}{0.15\textwidth}
        \includegraphics[width=\linewidth]{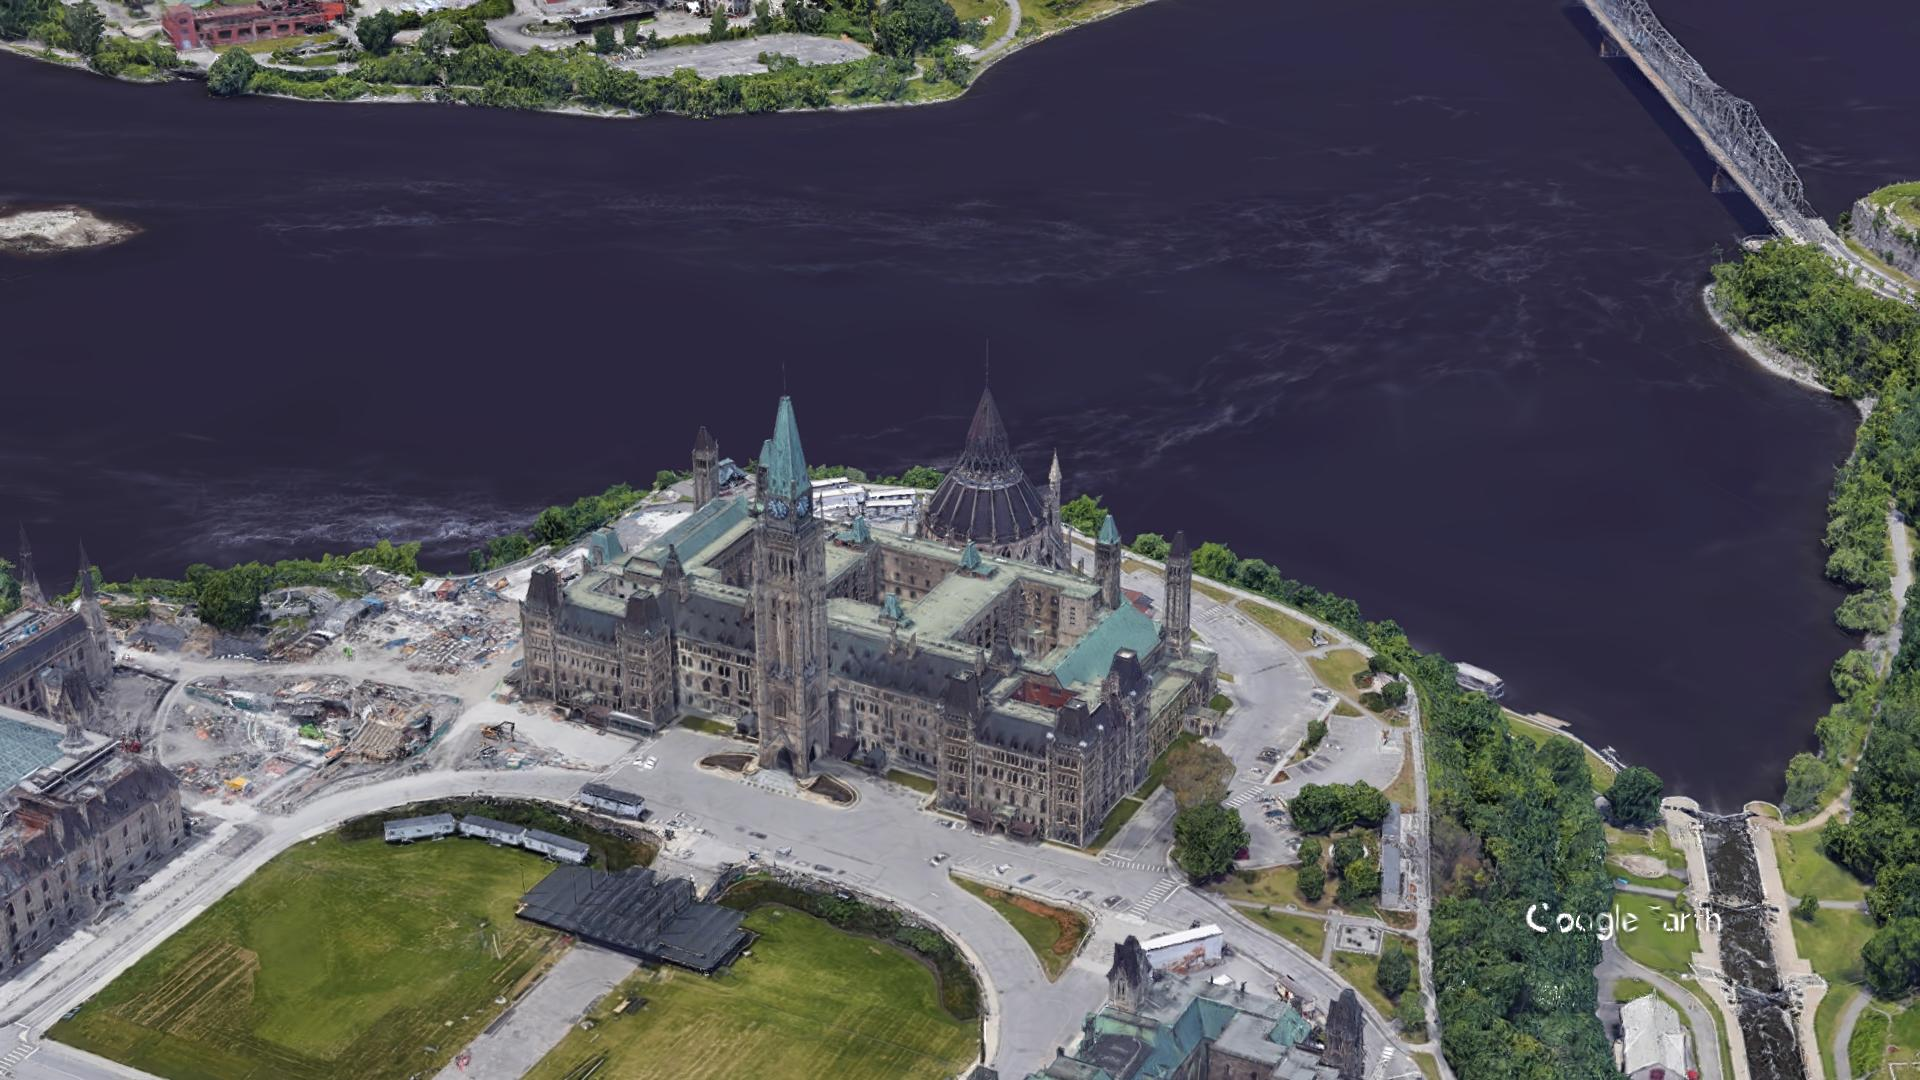}
    \end{subfigure}
    \begin{subfigure}{0.15\textwidth}
        \includegraphics[width=\linewidth]{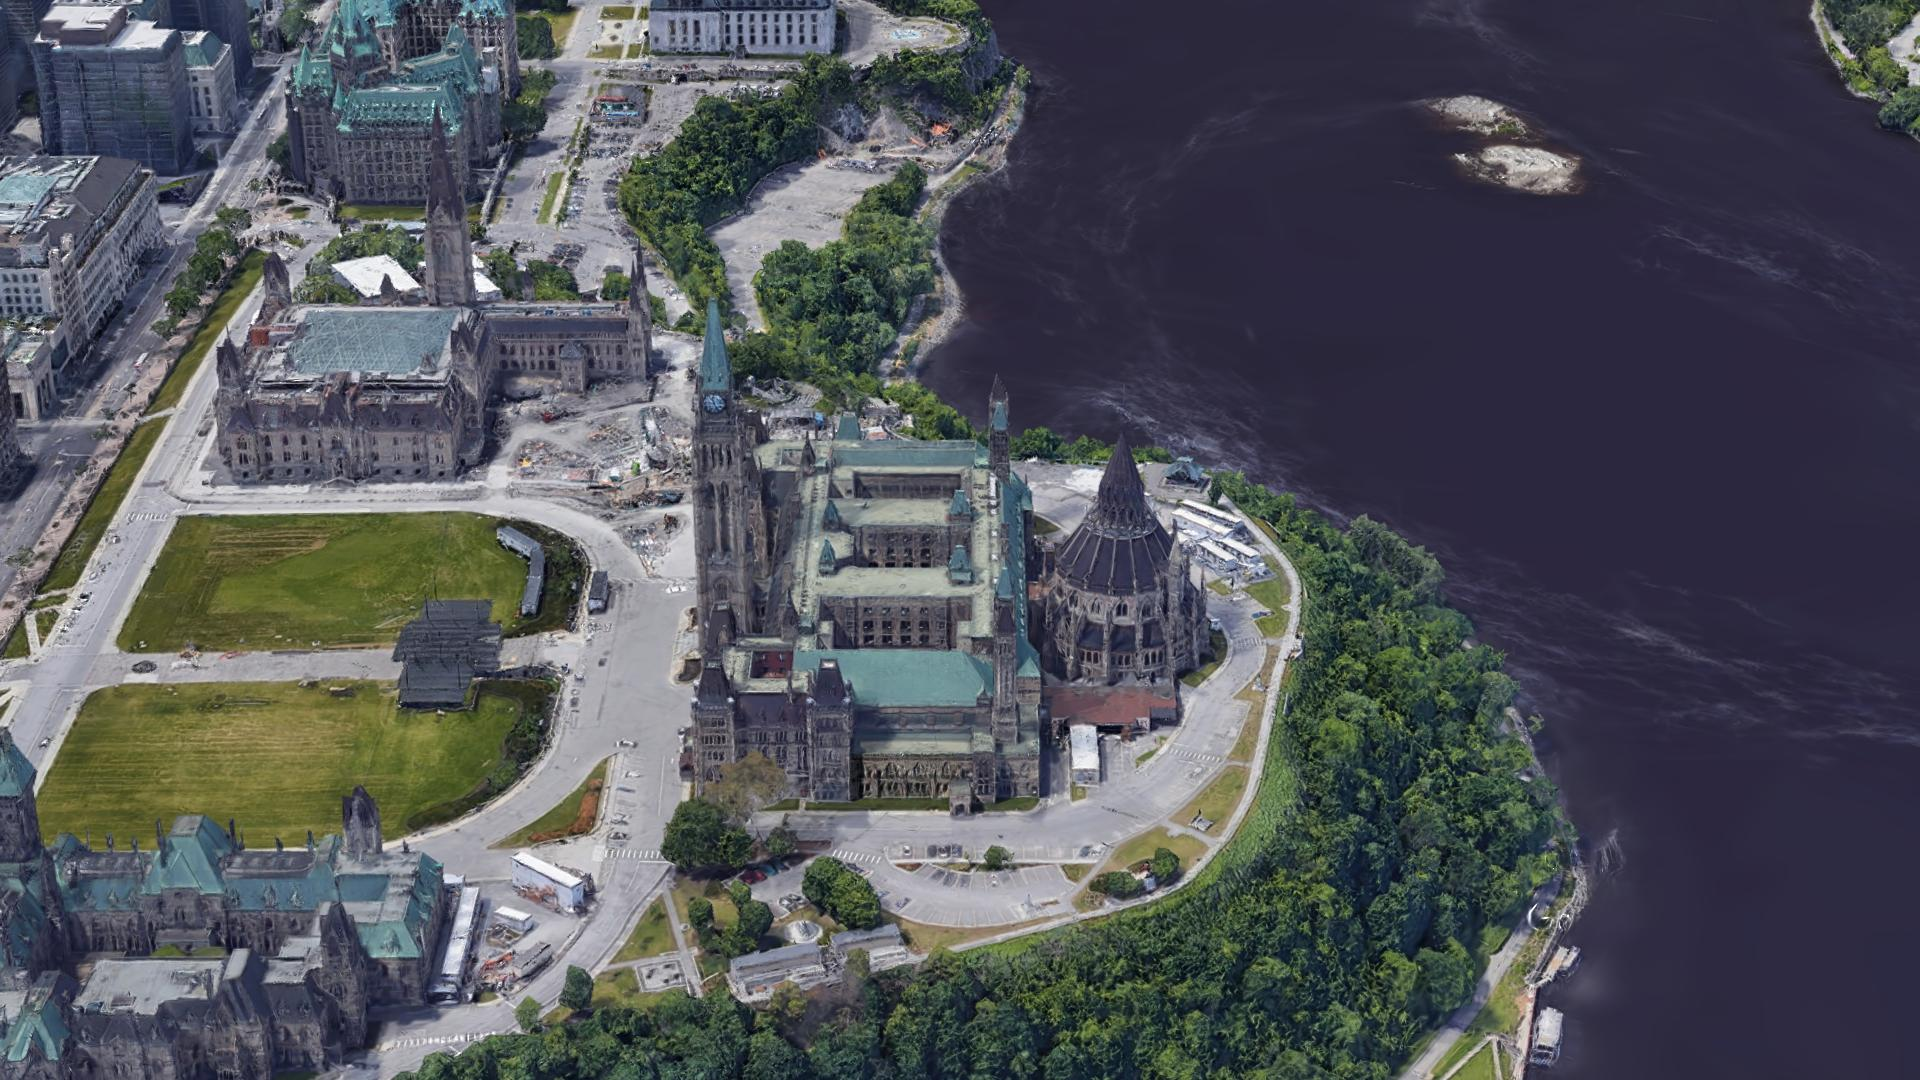}
    \end{subfigure}
    \begin{subfigure}{0.15\textwidth}
    \vspace{0.2cm}
        \includegraphics[width=\linewidth]{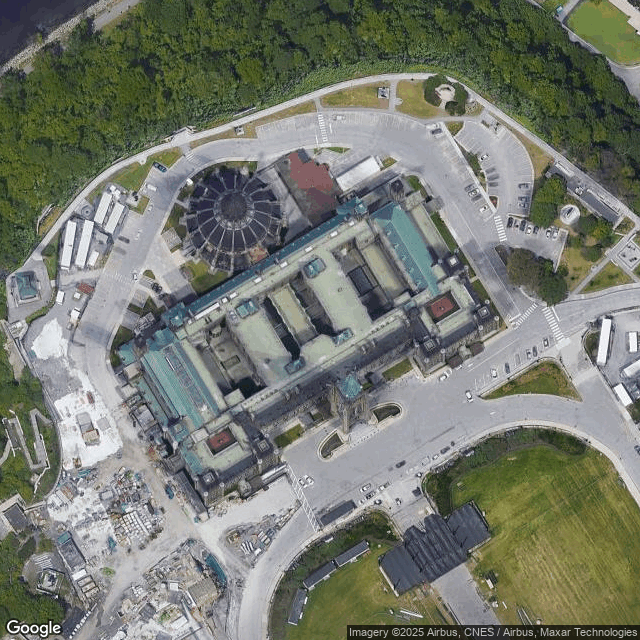}
    \end{subfigure}
    \hspace{0.015\textwidth}
    \begin{subfigure}{0.15\textwidth}
        \includegraphics[width=\linewidth]{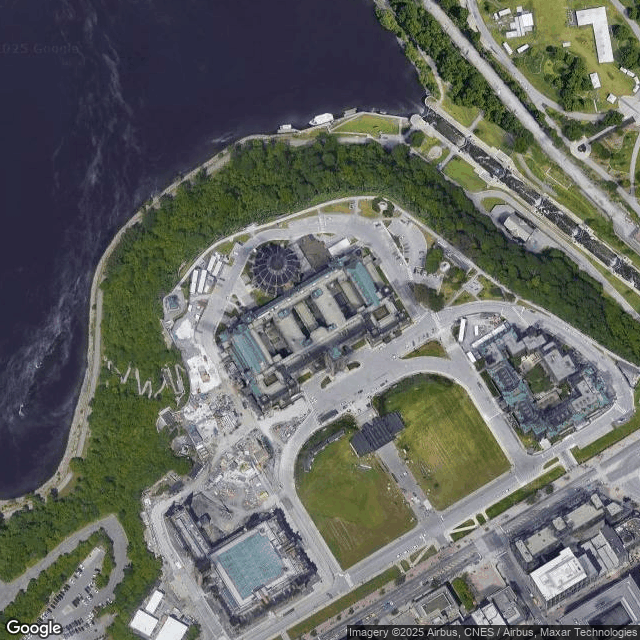}
    \end{subfigure}
    \caption{Parliament Hill of Canada input images. Top six: multi-view images (Google Earth Studio). Bottom two: multi-scale images (Google Maps Platform).}
    \label{fig:parliament_hill}
\end{figure}

\begin{figure}[h]
\vspace{-6.5cm}
    \centering
    \begin{subfigure}{0.15\textwidth}
        \includegraphics[width=\linewidth]{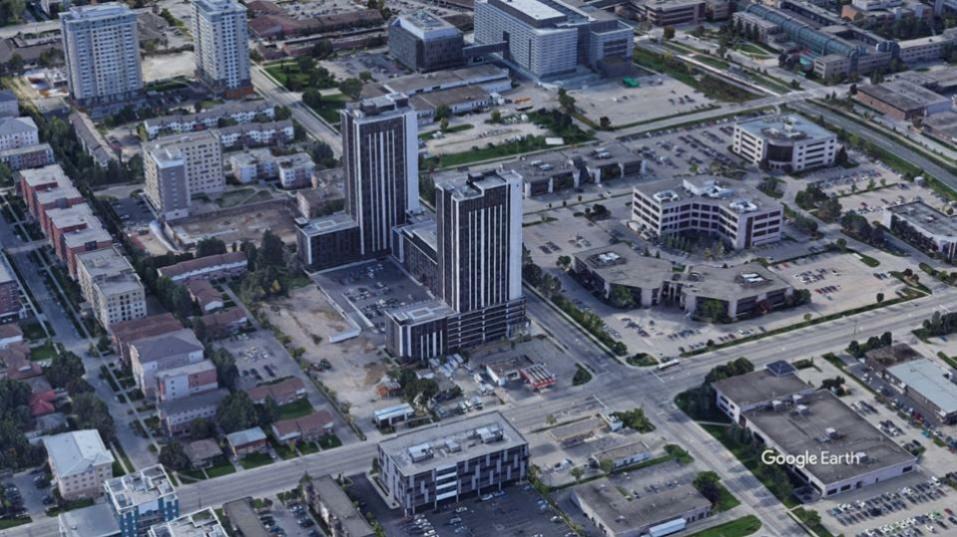} 
    \end{subfigure}
    \begin{subfigure}{0.15\textwidth}
        \includegraphics[width=\linewidth]{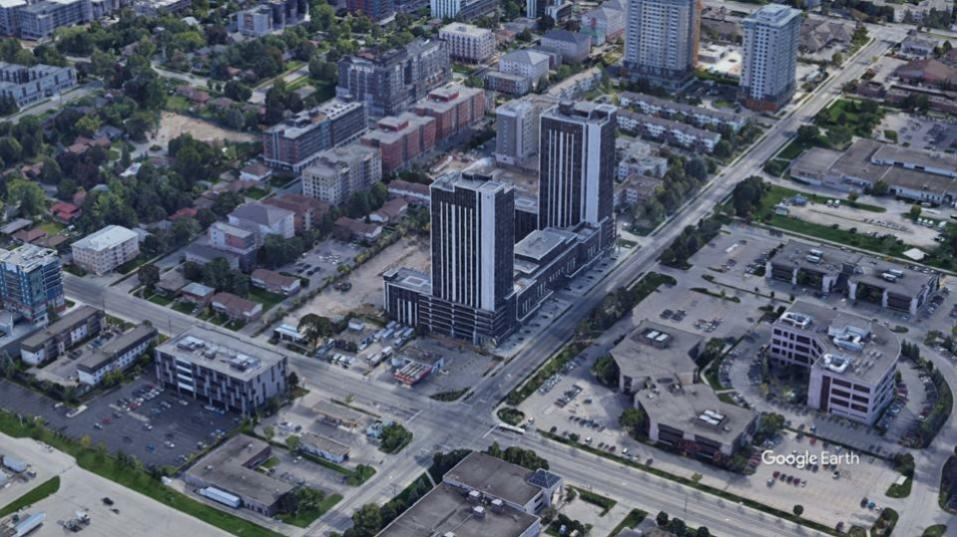}
    \end{subfigure}
    \begin{subfigure}{0.15\textwidth}
        \includegraphics[width=\linewidth]{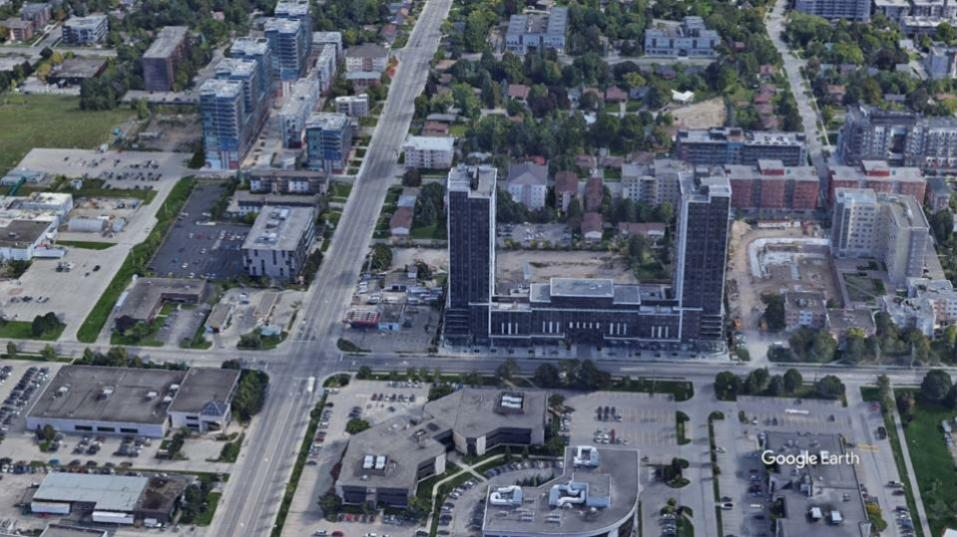}
    \end{subfigure}
    \\
    \begin{subfigure}{0.15\textwidth}
        \includegraphics[width=\linewidth]{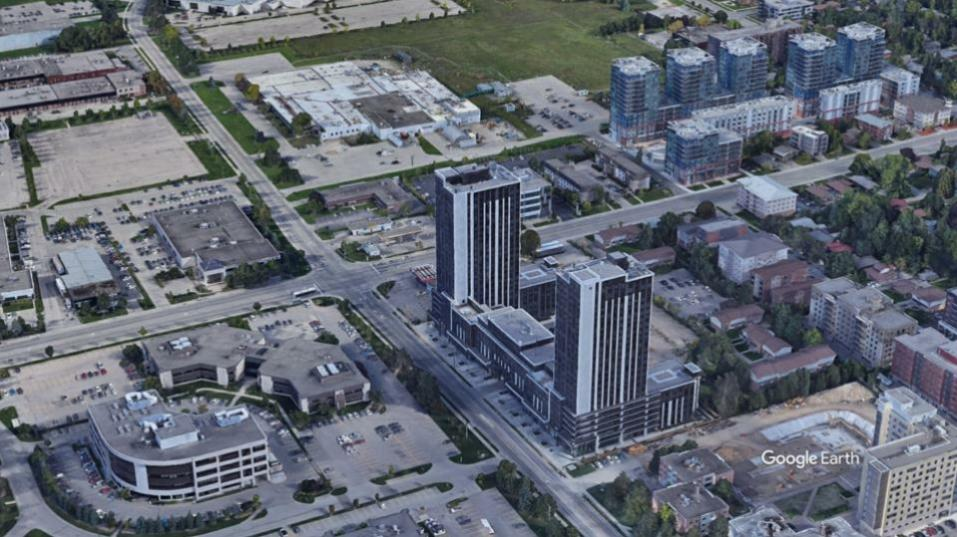}
    \end{subfigure}
    \begin{subfigure}{0.15\textwidth}
        \includegraphics[width=\linewidth]{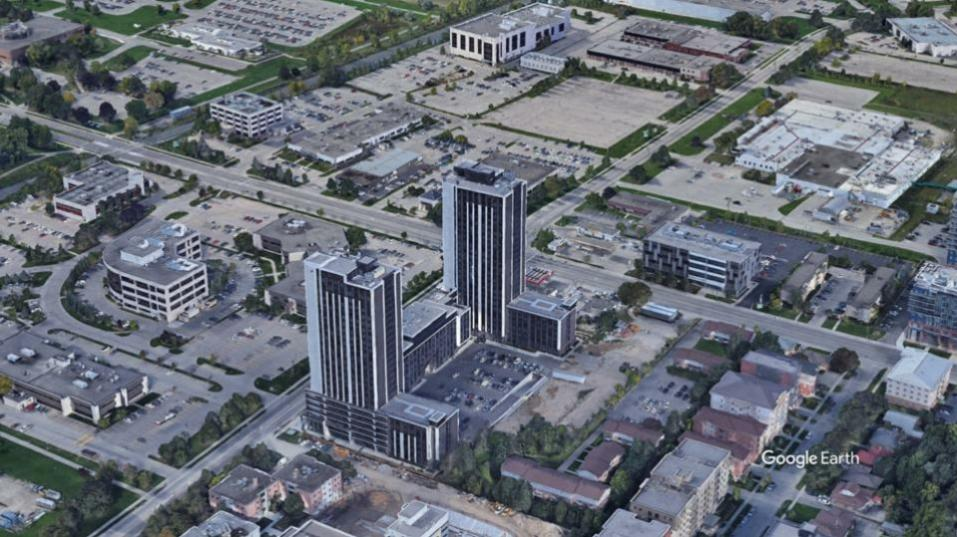}
    \end{subfigure}
    \begin{subfigure}{0.15\textwidth}
        \includegraphics[width=\linewidth]{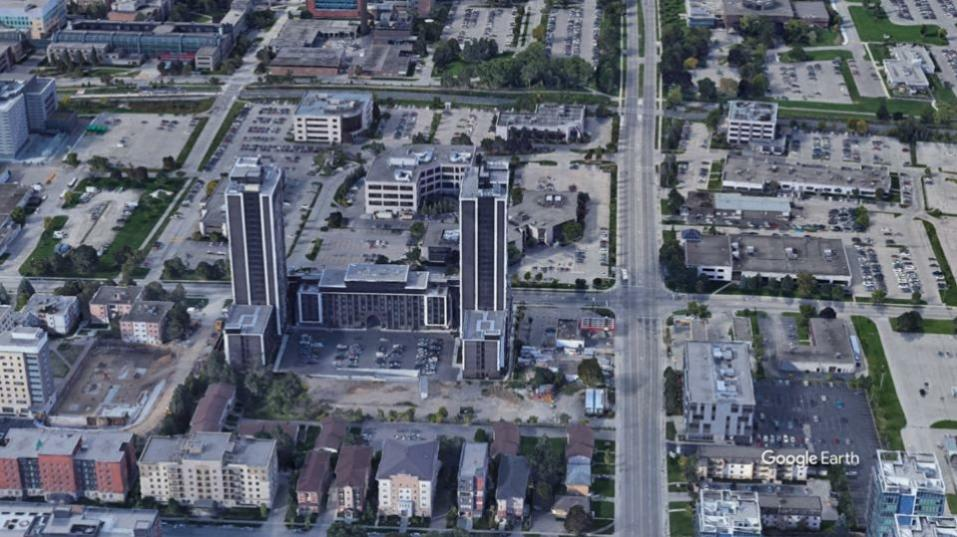}
    \end{subfigure}
    \begin{subfigure}{0.15\textwidth}
    \vspace{0.2cm}
        \includegraphics[width=\linewidth]{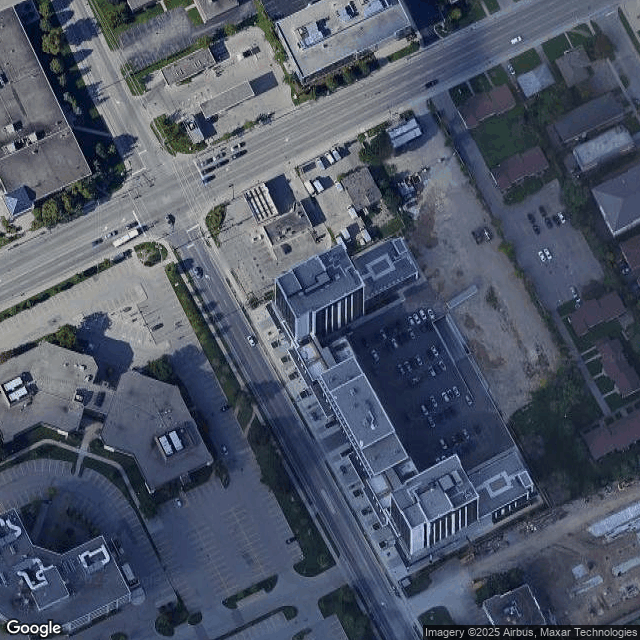}
    \end{subfigure}
    \hspace{0.015\textwidth}
    \begin{subfigure}{0.15\textwidth}
        \includegraphics[width=\linewidth]{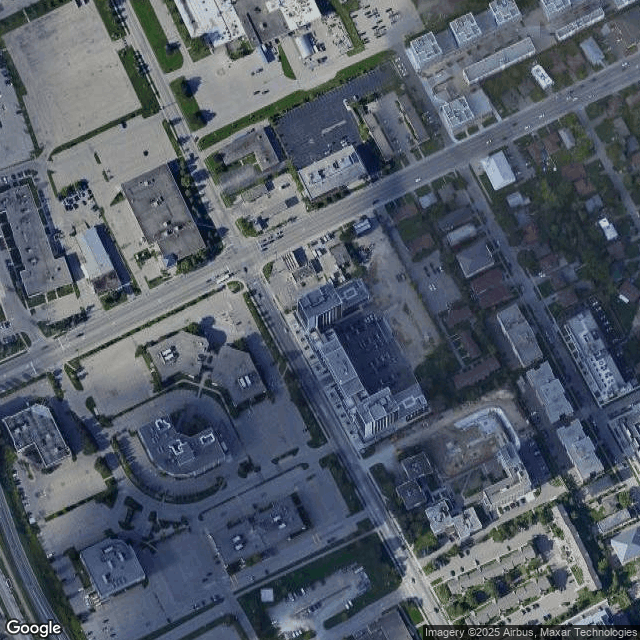}
    \end{subfigure}

    \caption{ICON building complex input images. Top six: multi-view images (Google Earth Studio). Bottom two: multi-scale images (Google Maps Platform).}
    \label{fig:icon}
\end{figure}
